# Supplementary material for: Velocity dependence of kinetic friction by multi-scale Quantum Mechanics/Green's Function molecular dynamics
Source: arXiv:2511.19222 ancillary file (2025-11-24)
Supplement: Supplementary file 1 [file GF_Velocity_SI.pdf]

# Supplementary Information
# Velocity dependence of kinetic friction by multi-scale Quantum Mechanics/Green's Function molecular dynamics

Alberto Pacini,[1,*] Seiji Kajita,[2,†] Gabriele Losi,[3] and Maria Clelia Righi[1,‡]

[1] *Department of Physics and Astronomy, University of Bologna, 40127 Bologna, Italy*
[2] *Toyota Central R&D Labs., Inc., 41-1, Yokomichi, Nagakute, Aichi, 480-1192, Japan*
[3] *Department of Physics, Mathematics and Informatics, University of Modena and Reggio Emilia, 41125 Modena, Italy*

## I. STATIC CALCULATION OF THE PES

We calculated the potential energy surfaces (PES) under load for the three diamond interfaces considered in the dynamic simulations. A load of 5 GPa was applied to the atoms of the topmost and bottomost layers of the two mating slabs. The system was then relaxed for different relative lateral positions of the two slabs, keeping fixed the lateral,$xy$, coordinates and optimizing the vertical one. The lateral positions were chosen by employing a $6\times10$ point grid, obtained by dividing the edges of the cell into approximately equally spaced sections. A radial basis function is then used to interpolate the calculated energies on the grid. The obtained PESes are reported in Fig. 1 on a common energy scale. The minimum energy paths (MEPs) for the different energy landscapes shown on the PES plots are calculated by employing the zero-temperature string method.[1]

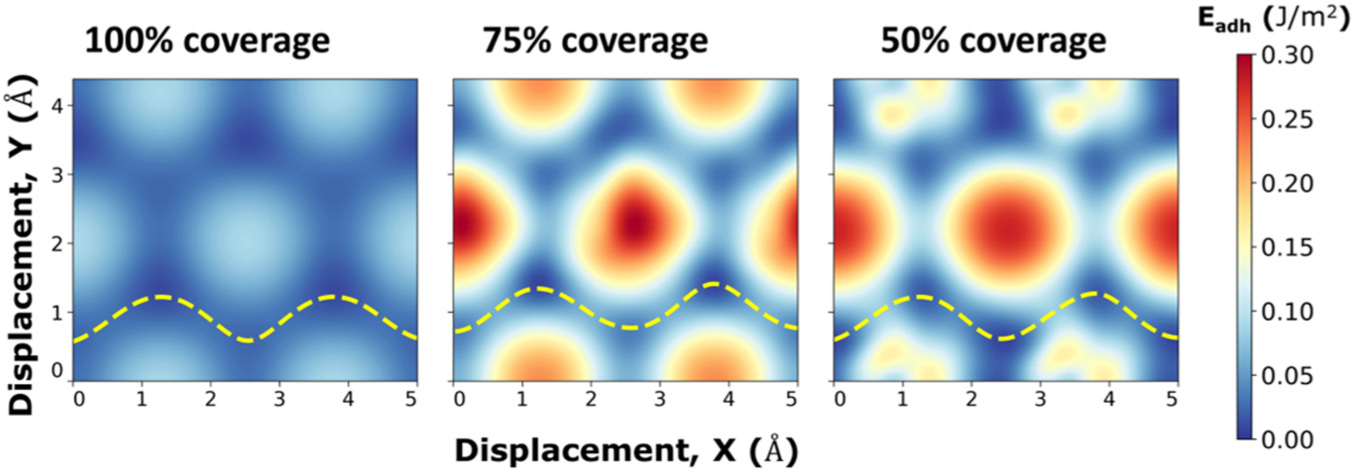


FIG. 1. PESes of the three systems under study in presence of a load of 5 GPa. The calculated MEPs are superimposed on the energy landscape as yellow dashed lines.

| Quantities derived from the PES | | | | |
|---|---|---|---|---|
| $\theta$ | $\tau_5$ | $\tau_1$ | $\tau_{mep}$ | $\mu_s$ |
| 100% | 0.87 | 0.90 | 0.3 | 0.06 |
| 75% | 2.56 | 2.80 | 1.12 | 0.22 |
| 50% | 2.65 | 2.84 | 1.51 | 0.28 |

TABLE I. Static properties of the three passivated interfaces. Hydrogen coverage, $\theta$, maximum resistance to sliding encountered along the dynamical trajectories at the two different applied shear stresses of 5 and 1 GPa, $\tau_{1,5}$, shear strength along the MEP, $\tau_{mep}$, and static friction coefficient $\mu_s$.

* alberto.pacini3@unibo.it
† fine-controller@mosk.tytlabs.co.jp
‡ clelia.righi@unibo.it

The calculated values for the maximum resistance to sliding along the paths followed during the dynamic simulations at different applied shear stresses $(\tau_1, \tau_5)$ and along the MEP $(\tau_{MEP})$ are reported in Tab.I. The static friction coefficient $\mu_s$, is calculated as the ratio of $\tau_{MEP}$ and the applied load, for the three passivated interfaces. As expected, the ideal shear strengths and static friction coefficients depend on the surface passivation. In particular, they increase for decreasing hydrogen coverage indicating the importance of the adhesive contribution to friction in the static regime.

## II. FORCE SIGNALS AND SPECTRAL ANALYSIS

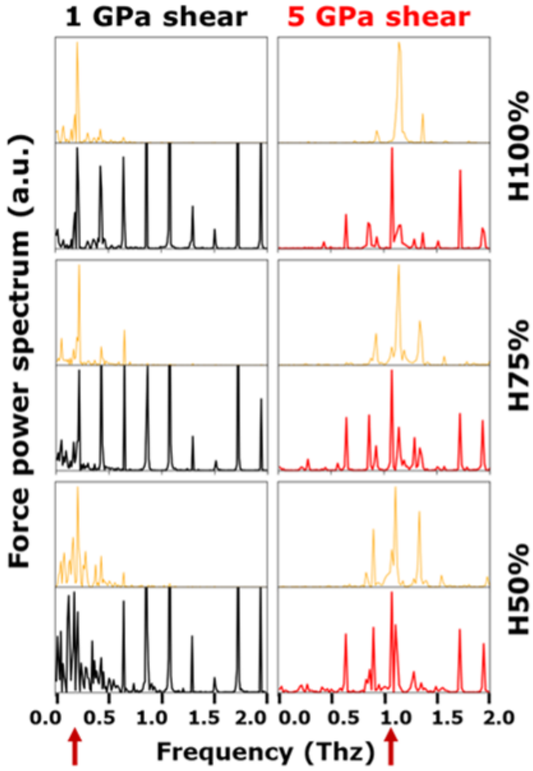


FIG. 2. Spectral intensity of the dynamical forces obtained from GF/QM MD simulations for *stick-slip* (black) and *continuous* (red) regimes, compared to $\tau_{PES}$ (orange) derived from super-imposing the dynamical trajectory on the static PES. Red arrows indicate the calculated washboard frequencies for both sliding regimes.

Fig.2 shows the spectral intensity of the lateral shear signals. The tree main rows refer to the three systems at different hydrogen passivation, while the columns refer to the two investigated sliding regimes with 1 GPa (*stick-slip*) and 5 GPa (*continuous sliding*) external applied shears. Each quadrant of the graph is composed of two paired plotted curves. The black or red curves (depending on the sliding regime) represent the spectra of the shear on the GF atoms measured during the QMGF simulation, while the orange curves are the spectra of the shear signals, obtained as the gradient along the dynamical trajectories on the PES. Red arrows at the bottom indicate the expected *washboard* frequencies for the two sliding regimes: $\nu_{\mathrm{wash}}^{1GPa}(\nu_{\mathrm{wash}}^{5GPa}) = 0.19(1.12)\ \mathrm{T}hz$. The spectra of the dynamical signal (black and red curves) resemble those of the PES-induced ones. Both signals are peaked near the *washboard* frequency while high-order harmonics are also present for the dynamical forces. The low-frequency region is dependent upon the degree of surface passivation and its width increases with decreasing hydrogen coverage. This low-frequency broadening causes an higher average of the friction force, consistent with the values reported in the main manuscript.

## III. COMPUTATIONAL DETAILS

The internal force matrix $D$ is calculated by static *ab initio* calculations of the diamond bulk, based on density functional theory (DFT) and a DFT linear-response approach to phonons calculation [2], performed with the pw.x and ph.x solvers from the Quantum Espresso package [3–5]. The Perdew, Burke, and Ernzerhof generalized gradient

approximation is used for the exchange-correlation functional [6]. Electronic wave functions are expanded on a plane-wave basis set with a cutoff energy of 25 Ry, and ionic species are described by ultra-soft pseudopotentials [7]. The matrix is approximated so that it only contains elements related to the nearest-neighbor interactions. The off-diagonal elements of the directional indices are also eliminated for the sake of numerical simplicity.

For the add-remove method, the classical force field of the $C_{link}$-$C_{GF}$ bond is set at the value of the corresponding element of the internal force matrix. The $C_{link}$-$H_{cap}$ spring constant is estimated from *ab initio* static calculations performed on a fully H-terminated 2×1 (111) diamond slab of 12 atomic layers. The estimated spring constant of the surface normal direction is 0.2575 Ht/bohr, while for the surface lateral direction is 0.0365 Ht/bohr. The stable bond length of $C_{link}$-$H_{cap}$ is $r_{eq} = 2.1043$ bohr.

We implemented the QMGF MD hybrid method into the Car-Parrinello solver cp.x. Time development of cp.x is solved by the Verlet method, which does not use velocities of atoms explicitly. On the other hand, the GF MD uses the general solutions to impose the temperature and stress by adding the velocity corrections $\mathbf{v}_T$ and $\mathbf{v}_S$. In order to merge the velocity correction into the QM MD algorithm, we used the leap-frog method that explicitly leverages the velocity term but is compatible to the Verlet method, as follows.

$$\begin{aligned}
\mathbf{p}_{\mathrm{GF}}(t+\frac{h}{2}) &\leftarrow \mathbf{p}_{\mathrm{GF}}(t-\frac{h}{2}) + h\mathbf{f}_{\mathrm{GF}}(t) \\
\mathbf{v}_{\mathrm{GF}}(t+\frac{h}{2}) &\leftarrow M^{-1}\mathbf{p}_{\mathrm{GF}}(t+\frac{h}{2}) + \mathbf{v}_T(t) + \mathbf{v}_S \\
\mathbf{r}_{\mathrm{GF}}(t+h) &\leftarrow \mathbf{r}_{\mathrm{GF}}(t) + h\mathbf{v}_{\mathrm{GF}}(t+\frac{h}{2}),
\end{aligned}$$

where $\mathbf{p}_{\mathrm{GF}}, \mathbf{v}_{\mathrm{GF}}$, and $\mathbf{r}_{\mathrm{GF}}$ are momentum, velocity, and position vectors of the GF MD atoms respectively. The time step is set to $h = 0.1$ fs, and the GF convolution integral used to evaluate the reduced force $\mathbf{f}_{\mathrm{GF}}$ is calculated based on a fast convolution method by employing a modified Talbot's Inverse Laplace Transform (mTILT). The parameters of mTILT are $B = 11$ and $N = 60$, equivalent to 121 integral points in the contour integral. The singular points of the Green's function are searched by evaluating its first and second derivatives on the imaginary axis. In the refresh treatment, we use $t_{\mathrm{refresh}} = 50,000h$, the anchor spring constant is 0.05 Ht/bohr for all the x, y, and z directions, and the relax time is $2,000h$. Temperature is set to 300 K by the thermostat of the GF MD method. The QM ions are thermalized by applying a Nosé-Hoover thermostat with a frequency of 80 Thz and imposing an average electronic kinetic energy of 0.25 atomic units on the electron degrees of freedom. The electronic mass and the time step of the molecular dynamics are selected to be 100 and 4 atomic units, respectively. At the beginning of our dynamic simulations, the CP solver is employed to obtain the ground state energy of the electronic wave functions with the steepest descent algorithm. Subsequently, the hybrid QMGF MD code is used to carry out the dynamic simulation. The computational parameters adopted for the CP scheme have been carefully selected to achieve good accordance between the temperatures of the QM and GF atoms during the dynamics for the system under study.

[1] W. E, W. Ren, and E. Vanden-Eijnden, The Journal of Chemical Physics **126**, 164103 (2007), https://doi.org/10.1063/1.2720838.

[2] P. Giannozzi, S. De Gironcoli, P. Pavone, and S. Baroni, Physical Review B **43**, 7231 (1991).

[3] P. Giannozzi, S. Baroni, N. Bonini, M. Calandra, R. Car, C. Cavazzoni, D. Ceresoli, G. L. Chiarotti, M. Cococcioni, I. Dabo, *et al.*, Journal of physics: Condensed matter **21**, 395502 (2009).

[4] P. Giannozzi, O. Andreussi, T. Brumme, O. Bunau, M. B. Nardelli, M. Calandra, R. Car, C. Cavazzoni, D. Ceresoli, M. Cococcioni, N. Colonna, I. Carnimeo, A. D. Corso, S. de Gironcoli, P. Delugas, R. A. DiStasio, A. Ferretti, A. Floris, G. Fratesi, G. Fugallo, R. Gebauer, U. Gerstmann, F. Giustino, T. Gorni, J. Jia, M. Kawamura, H.-Y. Ko, A. Kokalj, E. Küçükbenli, M. Lazzeri, M. Marsili, N. Marzari, F. Mauri, N. L. Nguyen, H.-V. Nguyen, A. O. de-la Roza, L. Paulatto, S. Poncé, D. Rocca, R. Sabatini, B. Santra, M. Schlipf, A. P. Seitsonen, A. Smogunov, I. Timrov, T. Thonhauser, P. Umari, N. Vast, X. Wu, and S. Baroni, Journal of Physics: Condensed Matter **29**, 465901 (2017).

[5] P. Giannozzi, O. Baseggio, P. Bonfà, D. Brunato, R. Car, I. Carnimeo, C. Cavazzoni, S. de Gironcoli, P. Delugas, F. Ferrari Ruffino, A. Ferretti, N. Marzari, I. Timrov, A. Urru, and S. Baroni, The Journal of Chemical Physics **152**, 154105 (2020).

[6] J. P. Perdew, K. Burke, and M. Ernzerhof, Physical review letters **77**, 3865 (1996).

[7] D. Vanderbilt, Physical review B **41**, 7892 (1990).
